# Supplementary material for: Siamese Contrastive Embedding Network for Compositional Zero-Shot Learning
Source: arXiv:2206.14475 source file (2022-06-29)

## Cotton Shoes (Heels)

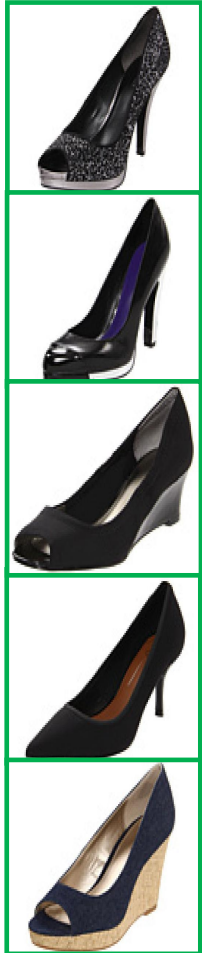

## Fleece Slippers

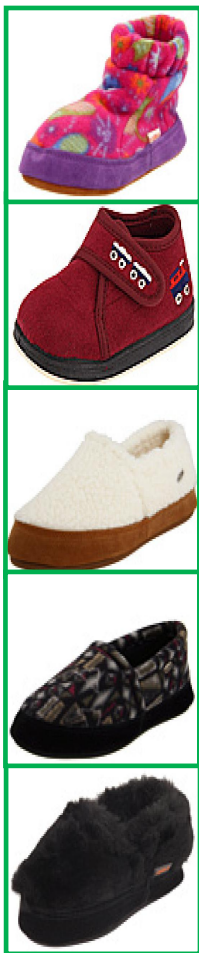

## Leather Sandals

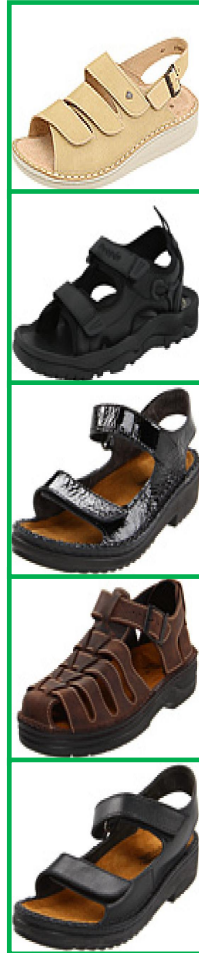

## Lace Sandals

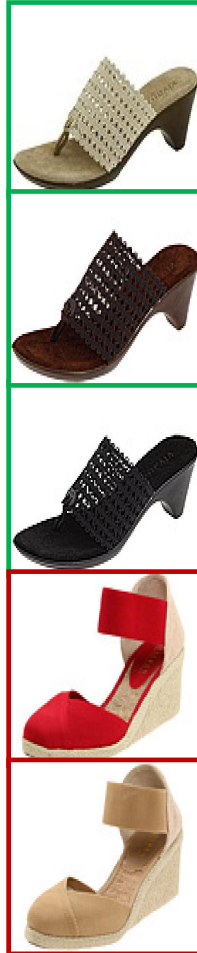

## Linen Sandals

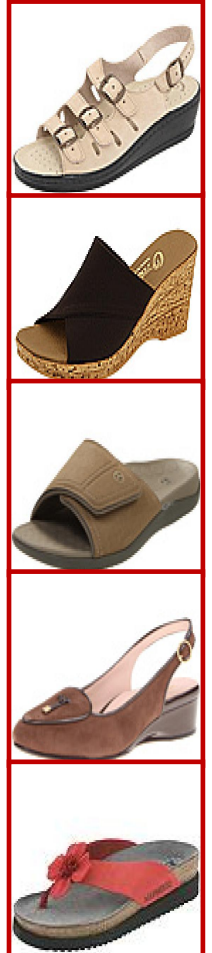

## Cotton Shoes (Heels)

## Fleece Slippers

## Leather Sandals

## lace sandals

## Linen Sandals

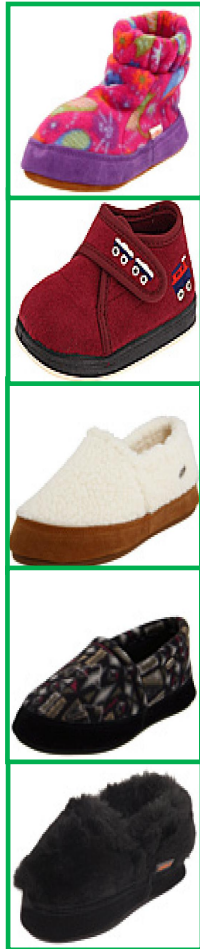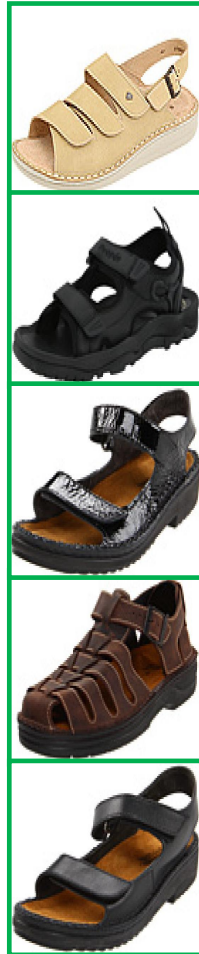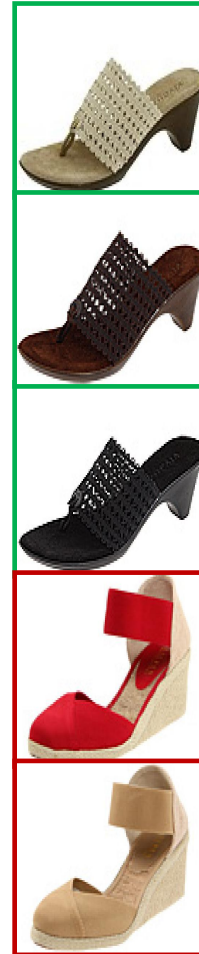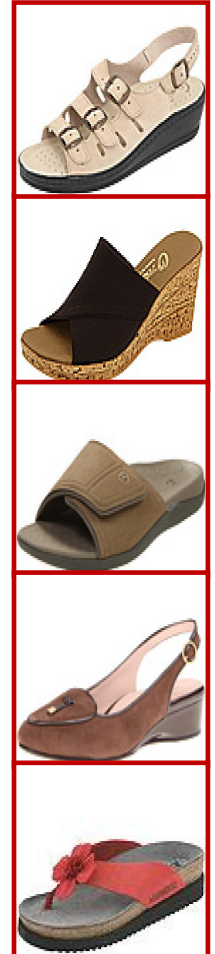

Supplement: Supplementary file 1 [file result-supp-2.pdf]
